# Supplementary material for: Conditional not displacement: fast multi-oscillator control with a single qubit
Source: arXiv:2301.09831 source file (2024-04-03)
Supplement: Supplementary file 1 [file supp.tex]

\section{The fast conditional displacement}
\subsection{QC mapping}
\subsection{simulations conditional displacements}
\subsection{Measurement of non local operators}
\subsection{Photon loss as limiting factor }
\subsection{MLE and fidelty}

\begin{table*}[htp!]

\centering
\begin{tabular}{ c | c c c c c c  }
\as{
   &  \boldsymbol{$\omega/2\pi$}  &  $\boldsymbol{Mode}$  &  \boldsymbol{$T_1$} & \boldsymbol{$T_2$} & \boldsymbol{$T^{E}_2$}  &  \boldsymbol{$\chi/2\pi$} \\
\hline
B & 6.56 GHz  &  TE102  &  60-62 $\mu s$  &  -  &  -  & 216-224 kHz \\
Bob   & 8.02 GHz  &  TE202 & 36-38  $\mu s$ & - & - & 31-36 kHz \\
Ancilla Transmon  &  5.37 GHz & - & 12-15  $\mu s$ & 5-7 $\mu s$ & 12-14 $\mu s$ & - \\
Mode Readout   & 4.02 & TE101  &  $\sim$ 600 ns & - & -  & $\sim$ 80 kHz\\
}
\end{tabular}
\caption{\textbf{afadfadf}}

\label{table:fidelty}
\end{table*}
